# Supplementary material for: LESA: Linguistic Encapsulation and Semantic Amalgamation Based Generalised Claim Detection from Online Content
Source: arXiv:2101.11891 source file (2021-01-28)
Supplement: Supplementary file 1 [file appendix.tex]

\section{Datasets}

There exist a few datasets for claim detection from online text (described later in this section). Most of them are formal structured texts. Unfortunately, none of the studies released the annotation guideline. A structured guideline is highly important for annotating a new dataset due to the subjectivity and high disagreement among  annotators. Moreover, to the best of our knowledge, there exists no dataset for detecting claims in unstructured noisy data from platforms like Twitter. Therefore, we collect our own dataset from multiple sources, form annotation guidelines and label a dataset of $9,894$ COVID-19 tweets.  In this section, we describe our data collection and annotation process, the challenges and the consolidated guidelines we form, various statistics of our dataset and the other existing datasets we use.

\subsection{Data Collection}

Multiple COVID-19 related tweets and datasets have been made public in recent times. However,  \cite{alam2020fighting} is the only one which released COVID-19 related claims, but that too in very less quantity (only $504$ tweets). They classified tweets as factually verifiable claims and non-factually verifiable claims, which is only a subset of the claims that exist. CLEF-2020 challenge by CheckThat! Lab also released two datasets that are of relevance \cite{10.1007/978-3-030-45442-5_65} -- Task 1 released $1,060$ COVID-19 tweets with $704$ claims and $356$ non-claims; Task 2 released a set of $1,000$ claims for claim retrieval. Due to the small size of these datasets, we resorted to COVID-19 Twitter datasets that have been made public on Kaggle; among them we used the datasets released by \cite{kaggleCarl}, \cite{kaggleShane}, and \cite{kaggleSVEN}. Additionally, there exist a few publicly available datasets containing COVID-19 related tweet IDs being released everyday in chronological order. We collected the tweet IDs from \citep{gitEchen} and \citep{QCRI}, hydrate\footnote{https://github.com/DocNow/hydrator} available tweets from these tweet IDs for annotation.

% \hl{1. If we did some preprocessing/cleaning mention it.}\\
% \hl{2. Data annotation guideline section before data annotation}

\subsection{Data Preprocessing}
Our pre-processing stage involves
 removing hashtags, URLs, user handles and non-ASCII characters. All tweets with character count less than $20$ and word count less than 4 are also removed, owing to the lack of context for their interpretation. Finally, we spell-check the words using symspellpy\footnote{https://pypi.org/project/symspellpy/}. The final dataset contains $9,894$ tweets which were split into 70\% for training, 10\% for validation and 1\% for testing. 

\subsection{Data Annotation Guidelines}

Our official definition adopted for claims is to {\em state or assert that something is the case, with or without providing evidence or proof}. Following are our guidelines for what qualifies as a claim. Anything that does not qualify as a claim, is labelled as `non-claim'. However, certain clarifying guidelines are also given for non-claims.

Note that some guidelines for claims also contain situations (with examples) where the guidelines do not generalise and input is labelled non-claim; vice versa also holds. Such exceptions are preceded by an asterisk (*).

\textit{Labels}: The tweets are labelled 1 for claim, 0 for non-claim and x in obscure situations. This is considered only when the language of the tweet is incomprehensible or if no guideline can be referred to annotate it.\\

% \subsection{Guidelines for claims}
\subsection{Guidelines for claims}
% \hl{1. For each point, move example on a separate line. It should be clear that what is guideline and which one is an example.} \\
% \hl{2. Also, highlight/underline the target phrases.}
% \hl{3. Make is itemize not enumerate.}
% \hl{4. Change begin quote (") with (``).}

%%%%%%%%%%%%%%%%%%%%%%%%%% Claim guideline table %%%%%%%%%%%%%%%%%%%%%%%%%%%%%%
%\if0
\begin{table*}[ht!]
 \centering
 \resizebox{\textwidth}{!}{
 \begin{tabular}{l|p{30em}}
 \bf Guideline & \bf Examples  \\ 
 
 \hline
 \multirow{1}{*}{\parbox{6cm}{Tweets mentioning \underline{statistics, dates} \underline{ or numbers}.}} & \textit{[``just 1 case of corona virus in india and people are crazy for masks daily 400 people die in road crashes still no craze for helmetsthinking face safetysaves be it virus or road crashes"]} \\ 
 
 \hline
 \multirow{1}{*}{\parbox{6cm}{Tweets mentioning a \underline{personal} \underline{experience.}}} & \textit{[``i live in seattle i have all symptoms of covid19 and have a history of chronic bronchitis since i work in a physical therapy clinic with many 65 patients and those with chronic illnesses i decided to be responsible and go to get tested this is how that went"]} \\ 

 \hline
 \multirow{1}{*}{\parbox{6cm}{Tweets \underline{‘reporting’ something to be } \underline{true} or an instance to have happened or will happen.}} & \textit{[``breaking boris johnson says he visited kettering hospital shook hands with corona patients but the hospital doesnt have corona cases shaking hands would be dangerous not sure how ill gloss over the fact the pm is a liar a complete fucking idiot but ill find a way x"]} \\ 

 \hline 
  \multirow{3}{*}{\parbox{6cm}{Tweets containing \underline{verified facts} also account for a claim, a veracious claim that is. (\textit{Note}: a fact known by one, may not necessarily be known by another)}}  & \textit{[``The Chinese CDC has started research and development of a vaccine for the \#coronavirus.”]}\\
  & \\
  & \\
    
 \hline 
 \multirow{2}{*}{\parbox{6cm}{Tweets that \underline{negate a possibly } \underline{false claim} are also accounted as claims.}} & \textit{[``disinfectants are not a cure for coronavirus”]} \\
 & \\
 & \\
 
\hline
\multirow{4}{*}{\parbox{6cm}{Tweets that \underline{indirectly (subtly) imply} that something is true.}} & \textit{[``b52questions 1 why is rudy not under arrest 2 why is harvey not in rikers 3 why is cuccinelli still working 4 has barr quit yet 5 when is flynn being sentenced 6 who trusts pence and mrs miller with messaging about coronavirus 7 are rs happy wtheir guy"]} \\ \cline{2-2}
& \textit{[``do rich people know theyll get the virus if poor people cant be tested and diagnoseddo rich people know theyll get the virus if poor people cant be tested and diagnosed"]} \\

\hline
\multirow{3}{*}{\parbox{6cm}{ Claims \underline{made in sarcasm or humour}.}} & \textit{[``@TheDailyShow Newsflash! \#trumpfact If you paint your face \#orange you will be \#immune to #coronavirus”]} \\ \cline{2-2}
& \textit{[``RT @\_saraellen: If you’ve ever used messers bathroom you’re immune to corona virus.”]}\\ \cline{2-2}
& \textit{[``corona virus minding its business by avoiding africa and going to other continents"]} \\
 
\hline
\multirow{2}{*}{\parbox{6cm}{All opinions are not claims. \underline{Opinions that have societal} \underline{implications} are considered as claims.}} & 
\textit{[``@derekgilbert I think the Chinese stole a bio weapon https://t.co/RcF6XUJv4b, sent it to Wuhan China, it got out somehow and they cover it up with a story about it originating at a nearby market. They know how bad the virus is and quarantine entire cities. https://t.co/ZwMqsiWGau"]} \\ \cline{2-2}
& \textit{[``I think Burger King fries are better than Mc'D's"]}\\

\hline
\multirow{2}{*}{\parbox{6cm}{Tweet that says something is true and provides an \underline{attachment} \underline{ as evidence or to support} \underline{the statement}.}} 
& \textit{[``RT @Jawn42: If you ate here growing up, you're immune to the Coronavirus. https://t.co/b9a0hm171b”]}\\ \cline{2-2}
& \textit{[``RT @TerminalLance: This kills Coronavirus in the system https://t.co/iOFNlkSrUj”]}\\ 

\hline
\multirow{1}{*}{\parbox{6cm}{A claim can be a sub-part of a question.}} & \textit{[``Does the pneumonia shot help protect from developing pneumonia caused by \#covid19”]} - the claim here being that pneumonia is caused by COVID-19.\\

\hline
\end{tabular}}
\caption{Guidelines for claims along with examples.}
\label{tab:guidelines:claim}
\end{table*}
%\fi
%%%%%%%%%%%%%%%%%%%%%%%%%%%%%%%%%%%%%%%%%%%%%%%%%%%%%%%%%%%%%%%%%%%%%%

\begin{itemize}
    \item Tweets mentioning \underline{statistics, dates or numbers}. \\
\textbf{Example:}    
\textit{[``just 1 case of corona virus in india and people are crazy for masks daily 400 people die in road crashes still no craze for helmetsthinking face safetysaves be it virus or road crashes"]}

    \item Tweets mentioning a \underline{personal experience}. \\
    \textbf{Example:} 
\textit{[``i live in seattle i have all symptoms of covid19 and have a history of chronic bronchitis since i work in a physical therapy clinic with many 65 patients and those with chronic illnesses i decided to be responsible and go to get tested this is how that went"]}

    \item Tweets \underline{‘reporting’ something to be true} or an instance to have happened or will happen. \\
    \textbf{Example:} 
\textit{[``breaking boris johnson says he visited kettering hospital shook hands with corona patients but the hospital doesnt have corona cases shaking hands would be dangerous not sure how ill gloss over the fact the pm is a liar a complete fucking idiot but ill find a way x"]}

    \item Tweets containing \underline{verified facts} also account for a claim, a veracious claim that is. \\
    (\textit{Note}: a fact known by one, may not necessarily be known by another)\\
    \textbf{Example:} 
\textit{[``The Chinese CDC has started research and development of a vaccine for the \#coronavirus.”]} - known fact

    \item Tweets that \underline{negate a possibly false claim} are also accounted as claims.\\
    \textbf{Example:} 
\textit{[``disinfectants are not a cure for coronavirus”]}

    \item Tweets that \underline{indirectly (subtly) imply} that something is true. \\
    \textbf{Example 1:} 
\textit{[``b52questions 1 why is rudy not under arrest 2 why is harvey not in rikers 3 why is cuccinelli still working 4 has barr quit yet 5 when is flynn being sentenced 6 who trusts pence and mrs miller with messaging about coronavirus 7 are rs happy wtheir guy"]} - indirectly implies rudy is not under arrest and harvey is not in rikers\\
\textbf{Example 2:} 
\textit{[``do rich people know theyll get the virus if poor people cant be tested and diagnoseddo rich people know theyll get the virus if poor people cant be tested and diagnosed"]} - indirectly implies rich people will get the virus if poor people can’t be tested

    \item Claims \underline{made in sarcasm or humour}.\\
    \textbf{Example 1:} 
\textit{[``@TheDailyShow Newsflash! \#trumpfact If you paint your face \#orange you will be \#immune to #coronavirus”]} \\
\textbf{Example 2:} 
\textit{[``RT @\_saraellen: If you’ve ever used messers bathroom you’re immune to corona virus.”]}\\
\textbf{Example 3:} 
\textit{[``corona virus minding its business by avoiding africa and going to other continents"]} \\
Example 1 and 2 are both examples of claims, even if evidently sarcastic. Example 3 is a humour oriented claim

    \item All opinions are not claims. \underline{Opinions that have societal implications} are considered as claims.\\
    \textbf{Example 1:} 
\textit{[``@derekgilbert I think the Chinese stole a bio weapon https://t.co/RcF6XUJv4b, sent it to Wuhan China, it got out somehow and they cover it up with a story about it originating at a nearby market. They know how bad the virus is and quarantine entire cities. https://t.co/ZwMqsiWGau"]} \\
% \textbf{{*}} However, not all opinions are claims. 
% \hl{Combine this sentence with the previous and try to explain as example 1 and example 2 in a single paragraph.}\\
\textbf{Example 2:} 
\textit{[``I think Burger King fries are better than Mc'D's"]}\\ 
Example 1 is a opinion that claims something to have happened, whose veracity will affect a certain section of the society. Example 2, on the other hand, is a personal belief that majorly impacts only the person making the tweet.  

    \item Tweet that says something is true and provides an \underline{attachment as evidence or to support the statement}. \\
    \textbf{Example 1:} 
\textit{[``RT @Jawn42: If you ate here growing up, you're immune to the Coronavirus. https://t.co/b9a0hm171b”]}\\
\textbf{Example 2:} 
\textit{[``RT @TerminalLance: This kills Coronavirus in the system https://t.co/iOFNlkSrUj”]}\\  \\
\textbf{{*}} However, if a person says something is provided in the attachment, that will not be a claim. \\
\textbf{Example:}
\textit{[``im stunned by the depth of coronavirus information being released in singapore on this website you can see every known infection case where the person lives and works which hospital they got admitted to and the network topology of carriers all laid out on a timeseries link"]}

    \item A claim can be a sub-part of a question. \\
    \textbf{Example:} 
\textit{[``Does the pneumonia shot help protect from developing pneumonia caused by \#covid19”]} - the claim here being that pneumonia is caused by COVID-19.
\end{itemize}
\\

%%%%%%%%%%%%%%%%%%%%%%%%% Non- Claim guidelines table %%%%%%%%%%%%%%%%%%%%%%%%%%
%\if0
\begin{table*}[ht!]
 \centering
 \resizebox{\textwidth}{!}{
 \begin{tabular}{l|p{30em}}
 \bf Guideline & \bf Examples  \\ \hline

 \multirow{4}{*}{\parbox{6cm}{Hoping that something happens or feeling something is true is not claiming it.}} & \textit{[``World doesn’t end if u don’t give your opinions about corona virus. I’m drinking  \#nilavembu boiled in hot water and hope it prevents. \#COVIDー19 \#coronapocolypse”]} \\ \cline{2-2}
 & \textit{[I feel like I’m immune to coronavirus.]}  \\

 \hline
 \multirow{4}{*}{\parbox{6cm}{Inclusion of words that project doubt over the said statement.}} & \textit{[\@politicalelle Political correctness infecting the \#Coronavirus . Let's change words describing the virus maybe that will cure it.]} \\ \cline{2-2}
 & \textit{[Coronavirus may have originated in lab linked to China's biowarfare program \#coronavirus https://t.co/2NSWidMkoa]}  \\ 

 \hline
\multirow{1}{*}{\parbox{6cm}{Urging one to not claim something or to spread misinformation is not a claim.}} & \textit{[\#Covid19 - Dear all: Stop telling the public that plaquenil/Azithromycine is a cure!!!!! Plz some leadership is needed regarding this matter!]} \\ %\cline{2-2}

 \hline 
\multirow{3}{*}{\parbox{6cm}{Questioning a possible claim is not a claim.}} & \textit{Do disinfectants really cure Corona?} \\ \cline{2-2}
 & \textit{[]Would you like to promote a cure that can kill 90\% \#COVIDー19 virus in the body in 3-15 min?]} \\
 
 \hline
 \multirow{1}{*}{\parbox{6cm}{Warning someone against a claim is not a claim.}} & \textit{[If you think drinking disinfectants will cure \#Covid\_19 , you deserve death \#trump]} \\ % \cline{2-2}

 \hline
\end{tabular}}
\caption{Guidelines for non-claims along with examples.}
\label{tab:guidelines:non-claim}
\end{table*}
%\fi
%%%%%%%%%%%%%%%%%%%%%%%%%%%%%%%%%%%%%%%%%%%%%%%%%%%%%%%%%%%%

\subsection{Guidelines for non-claims} 
% these guidelines are non-exhaustive (refer to Note 1)

\begin{itemize}
    \item Hoping that something happens or feeling something is true is not claiming it.\\
    \textbf{Example 1:} 
\textit{[``World doesn’t end if u don’t give your opinions about corona virus. I’m drinking  \#nilavembu boiled in hot water and hope it prevents. \#COVIDー19 \#coronapocolypse”]}\\
\textbf{Example 2:} 
\textit{[``I feel like I’m immune to coronavirus.”]}

    \item Inclusion of words that project doubt over the said statement.\\
    \textbf{Example:} 
\textit{[``\@politicalelle Political correctness infecting the \#Coronavirus . Let's change words describing the virus maybe that will cure it.”]}\\\\
\textbf{{*}} Tweets containing doubt-casting words can still, however, contain claims.\\
\textbf{Example:} 
\textit{[``Coronavirus may have originated in lab linked to China's biowarfare program \#coronavirus https://t.co/2NSWidMkoa”]}

    \item Urging one to not claim something or to spread misinformation is not a claim.\\
    \textbf{Example:} 
\textit{[``\#Covid19 - Dear all: Stop telling the public that plaquenil/Azithromycine is a cure!!!!! Plz some leadership is needed regarding this matter!”]}

    \item Questioning a possible claim is not a claim.\\
    \textbf{Example:} 
\textit{[``Do disinfectants really cure Corona?”]}\\\\
\textbf{{*}} However, a tweet containing a question can still comprise a claim.\\
\textbf{Example:} 
\textit{[``Would you like to promote a cure that can kill 90\% \#COVIDー19 virus in the body in 3-15 min?"]} - the tweet claims that there exists a cure that can kill 90\% of COVID-19 virus in the body

    \item Warning someone against a claim is not a claim.\\
    \textbf{Example:} 
\textit{[``If you think drinking disinfectants will cure \#Covid\_19 , you deserve death \#trump”]} - this tweet may be hate speech but is not claiming something to be true or untrue.
    
\end{itemize}

\subsection{Data Annotation}
Scarce work in this field has been conducive to almost no annotation guidelines. High degree of subjectivity and possibility of unconscious bias also makes it difficult to identify claims and ensure consistency. Therefore after numerous rounds of discussion with subject experts, researchers and lexicographers, we manifest our own set of data annotation guidelines. They are formed after considering our definition of claim, adopted from Oxford's definition of the word\footnote{https://www.lexico.com/definition/claim}, its semantics and syntactical implications and preview of existing guidelines available in claim detection datasets. %%%%

The guidelines were formed in four steps. Before the onset of annotation process, existing guidelines \cite{alam2020fighting} were read and their pertinence discussed. Then 3 annotators re-labelled a set of 400 tweets from the CLEF Task 1 dataset \cite{10.1007/978-3-030-45442-5_65}, with a kappa score of 0.46. It was evident from this step that claim detection is a tough task for human annotators too. This was followed by a series of formal meetings to discuss the linguistic semantics of claims and its adaptation for noisy texts like twitter. Each draft was followed by annotation of a few hundred fresh tweets and applicability of the guidelines is a new environment. External annotators were also considered in the process to get a neutral and objective perception. In each round, all disagreement tweets were discussed to form the consolidated list of the below mentioned guidelines.  

Each tweet in our corpus of 10,200 tweets has been annotated by at least two annotators, with an average inter-annotator kappa score of 0.62. In case of a disagreement, the third annotator was considered and majority vote was used as the label. It is also worth mentioning that since we form our own guidelines we re-annotate the datasets obtained from external sources mentioned in Data Collection to ensure coherence and conformity. 

\subsection{Data Statistics}
Data statistics related to the assimilated dataset are given in Table \ref{data stats twitter}. We find that on an average a tweet contains x sentences and \~{} 24 words. Additionally, quartile-wise character and the word count has been given in Table \ref{quartile info}. As opposed to the datasets (mentioned in Other Datasets) that have been released for claim detection, we attempt to have more claims than non-claims in the final dataset. This is reflected in the percentage of claims in the overall dataset. For creating the training and dev sets, we downsample to a 1:1 ratio between claims and non-claims. The rationale behind having more claims than non-claims is to prevent false negatives, which is more serious in case of claim detection.

\begin{table}[t]
\centering
% \smallskip
\resizebox{0.49\textwidth}{!}{
\begin{tabular}{l|l|l|l}
\bf Statistic & \bf Overall & \bf Train & \bf Test \\
\hline
\bf \#S/tweet & 1.36 & 1.36 & 1.39 \\ 
\bf \#Tokens & 18,694 & 17,447 & 5,171\\
% \#Words/sentences & \\
\bf \#W/tweet & 24.2 & 23.8 & 21.6\\
\bf \#Claims & 8,650 (87.42\%) & 7,354 (87.45\%) & 1,296 (87.27\%)\\

%\#Claims(train) & 1,055 (10.66\%)\\
%\#Claims(dev) & 106 (1.07\%)\\
% \#Claims(test) & 1,296 (13.09\%)\\
\end{tabular}}
\caption{Dataset Statistics for Tweets}
\label{data stats twitter}
\end{table}

\begin{table}[t]
\centering
% \smallskip
\resizebox{0.39\textwidth}{!}{
\begin{tabular}{l|l|l|l}
Quartile[\#W/Tweet] &  Overall &  Train &  Test  \\
\hline
0.25  &  12.0 & 13.0 & 12.0\\
0.50  &  21.0 & 21.0 & 19.0\\
0.75  &  34.0 & 34.0 & 31.0\\
\hline 
 Quartile[\#Ch/Tweet] &  Overall &  Train &  Test \\
\hline
0.25  &   70.0 & 72.0 & 67.0\\
0.50  &  116.0  & 120.0 & 105.0\\
0.75  &  194.0  & 198.0 & 174.0\\

\end{tabular}}
\caption{Quartile-wise Word and Character Count}
\label{quartile info}
\end{table}

\subsection{Other Datasets} \label{other datasets}

\begin{table*}[t]
\centering

% \hl{1. Rename corpus as dataset and merge reference column with it. 2. Add row for our dataset as well. 
% \hl{3. Add avg length for each case. 4. Also, mention the train and test distribution for the experiments.}}
\smallskip
\resizebox{\textwidth}{!}{
\begin{tabular}{l|l|l|l|l|l|l}
\bf Dataset & \bf Genre & \bf \#Tokens & \bf \#Claims & \bf\#Words/Row & \bf \#Train Samples (Claims\%) & \bf \#Test Samples (Claims\%)  \\ 
\hline
MT
% , \cite{peldszus-stede-2015-joint} 
& micro texts & 8,865 & 112 (24.94\%) & 19.74 & 401 (24.94\%) & 48 (25\%)  \\
PE
% , \cite{stab-gurevych-2017-parsing} 
& persuasive essays & 147,271 & 2,108 (29.62\%) & 20.69 & 6,384 (29.53\%) & 732 (30.46\%) \\
OC
% , \cite{6061427} 
& online comments & 125,677 & 703 (7.86\%) & 14.27 & 8,010 (7.78\%) & 794 (8.06\%) \\
VG
% , \cite{reed-etal-2008-language} 
& various genres & 60,383 & 563 (19.81\%) & 21.67 & 2,507 (19.74\%) & 278 (20.50\%) \\ 
WD
% , \cite{habernal-gurevych-2015-exploiting}
& web discourse & 84,817 & 211 (5.41\%) & 22.61 & 3,522 (5.40\%) & 235 (5.96\%) \\
WTP
% , \cite{article} 
& wiki talk pages & 189,140 & 1,138 (12.45\%) & 20.84 & 8,204 (12.55\%) & 864 (12.15\%)\\
TWR & Tweets & 18,694 & 8,650 (87.42\%) & 24.21 & 7,420 (85.34\%) & 1484 (86.52\%) \\ 
\end{tabular}}
\caption{Dataset statistics}
\label{table: data stats}
\end{table*}

Since we attempt to create a generalised model that is able to detect the presence of a claim in any online text, we accumulate, in addition to the twitter dataset, available datasets from a wide variety of online texts. Statistics of six such datasets are given in Table \ref{table: data stats}. These datasets include German microtexts (MT) formed by \cite{peldszus-stede-2015-joint}, 402 persuasive student essay (PE) corpus by \cite{stab-gurevych-2017-parsing}, online comments (OC) from blog threads of LiveJournal as given by \cite{6061427}, the AraucariaDB corpus \cite{reed-etal-2008-language} comprising of various genres (VG) like newspaper editorials, parliamentary records, or judicial summaries, web discourse (WD) corpus such as blog posts, or user comments given by \cite{habernal-gurevych-2015-exploiting} and Wikipedia talk pages (WTP) formulated by \cite{article}. All these datasets represent claims at a discourse level. The aforementioned datasets are predominantly used in argument mining and claim, evidence and premise detection and demarcation.

\begin{table*}[t]
\centering
% \smallskip
\resizebox{\textwidth}{!}{
\begin{tabular}{l||c|c|c|c|c|c|c|c|c|c|c|c|c|c||c|c}
   \multirow{3}{*}{\bf Models} & \multicolumn{2}{c|}{\bf Noisy} & \multicolumn{4}{c|}{\bf Semi-Noisy} & \multicolumn{8}{c||}{\bf Non-Noisy} & \multicolumn{2}{c}{\multirow{3}{*}{\bf Wt Avg}} \\ 
\cline{2-15}
 & \multicolumn{2}{c|}{Twitter} & \multicolumn{2}{c|}{OC} & \multicolumn{2}{c|}{WTP} & \multicolumn{2}{c|}{MT} & \multicolumn{2}{c|}{PE} & \multicolumn{2}{c|}{VG} & \multicolumn{2}{c||}{WD} & \multicolumn{2}{c}{} \\ \cline{2-15}
 & $m\text{-}F1$ & $c\text{-}F1$ & $m\text{-}F1$ & $c\text{-}F1$& $m\text{-}F1$ & $c\text{-}F1$& $m\text{-}F1$ & $c\text{-}F1$& $m\text{-}F1$ & $c\text{-}F1$& $m\text{-}F1$ & $c\text{-}F1$& $m\text{-}F1$ & $c\text{-}F1$   \\ \hline
 
\hline
POS-only [2-gram] &	0.41 &	0.59 &	\bf0.52 &	0.14 &	\bf0.54 &	0.23 &	0.42 & 0.00 & 0.43 & 0.06 &	\bf0.55 &	0.30 &	\bf0.50 & 0.09 & 0.47 & 0.47\\

POS-only [3-gram] & \bf 0.49 &	\bf 0.74 &	0.51 &	\bf0.17 &	0.49 &	\bf0.24 &	0.54 &	0.32 &	\bf0.51 &	\bf0.32 &	\bf0.55 &	\bf0.39 &	0.43 &	\bf0.10 & \bf0.50 & \bf0.62\\

POS-only [4-gram] & 0.23 &	0.23 &	0.50 &	0.05 &	0.53 &	0.14 &	\bf 0.61 &	\bf0.35 &	0.43 &	0.06 &	0.53 &	0.18 &	0.47 &	0.00 & 0.41 & 0.19 \\
\hline

\end{tabular}}
\caption{Macro F1 and claim-F1 for POS n-gram experiments. } %\hl{Arrange this as per Table 6. Noisy, non-noise, semi-noisy.}} 
\label{Table: POS n-gram}
\end{table*}

\input{tables/pos_transformer}

\input{tables/hyperparameters}

\input{tables/individual_results}
